# Supplementary material for: Multi-Task Combinatorial Bandits for Budget Allocation
Source: arXiv:2409.00561 source file (2024-08-31)
Supplement: Supplementary file 1 [file 6.Appendix1.tex]

\section{Posterior Updating}\label{sec:posterior_dist}

Recall that $\vx_{m,k}$ denotes all features related to the adline $k$ in campaign $m$. For simplicity of notations, we assume $K\equiv K_m$ for all $m\in[M]$. We further define $\vx_{m} = (\vx_{m,1},\cdots,\vx_{m,K})$ as all features involved in campaign $m$, and $\vX = (\vx_{1},\cdots,\vx_{M})$ as all features involved in all campaigns. Likewise, we denote $\vthe_{m,k} = (\theta_{m,k,1},\cdots, \theta_{m,k,N})^T$, $\vthe_{m} = (\vthe_{m,1}^T, \cdots, \vthe_{m,K}^T)^T$, and $\vthe = (\vthe_1^T, \cdots, \vthe_M^T)^T$.

Suppose at decision point $t$,  the $m(t)$th  campaign was involved in the posterior updating process. Define $a_{m,k,t}$ as the action selected for the $k$th adline at round $t$, and $\vY_{t}$ is a $K\times 1$ vector containing the observed reward for the $K$ selected base arms. Let $\vpsi_{t}=\{\phi(\vx_{m(t),k,t}, a_{m(t),k,t})\}_{1\leq k\leq K}$ be a $d \times K$-dimensional matrix containing features of all base arms offered at round $t$ after a general transformation $\phi(\vx,a)$. Subsequently, $\vPsi_{1:H}=(\vpsi_{1},\cdots,\vpsi_{H})$ is a $d \times KH$ matrix including all transformed features from round $1$ to round $H$. Likewise, $\vY_{1:H} = (\vY_{1}^{T},\cdots,\vY_{H}^{T})^{T}$ includes observed rewards of all base arms offered till round $H$. 

Then, we define an $MKN\times KH$-dimensional indicator matrix $\vZ_{1:H}$, such that the $(i,l)$-th entry of $\vZ_{1:H}$ denotes whether the $l$th observation belongs to the $i$th $(m,k,a)$ tuple. More specifically, $\{\vZ_{1:H}\}_{i,l}=\mathds{I}\{g(l) = i\}$, where the function $g(l)$ maps the $l$-th observation to its corresponding base arm index. For each observation $l$, let $m(l)$, $k(l)$, and $a(l)$ represent the indices of the campaign, ad line, and budget level, respectively. The mapping function is defined as $g(l) = (m(l)-1) \times KN + (k(l)-1) \times N + a(l)$.

For clarity, we do not consider the based arm corresponding to 0 budget in this derivation. In practice, our algorithm considers an additional base arm with 0 budget for each ad line. However, it is worth noting that only the observations with a non-zero budget can provide useful information in the posterior updating process.

According to the main paper, our Bayesian hierarchical model is defined as follows:
%\begin{comment}
%\begin{equation}\label{General-version}
%    \begin{alignedat}{2}
%        &\text{(Prior)} \quad
%        \quad\quad\quad \quad\quad \quad\quad  
%        f(x)&&\sim \mathcal{N}(\mu_{\vgamma}(x), k_{\vgamma}(x,x'))\\
        %&\text{(Generalization)} \quad
 %       \; \vthe_{m}\mid \vx_{m},\vgamma && = f(\vx_{m})+\delta_{m}, \forall m,k,n,  \\
  %      &\text{(Observation)} \quad
 %       \;\quad\quad \;   Y_{m,k,n,t}  &&=  \theta_{m,k,n} + \epsilon_{m,k,n,t}, \forall (k,n)\in A_{m,t},\\
%        &\text{(Reward)} \quad \quad\quad
%        \quad\quad \quad \; R_{m,t} &&= \sum_{(k,n)\in A_{m,t}}Y_{m,k,n,t},
%    \end{alignedat}
%\end{equation}
%\end{comment}

\begin{equation}\label{appendix:model}
            \begin{alignedat}{2}
            &\text{(Prior)} \quad \quad \quad \quad \quad
                \;    \text{Prior information Q} && \text{ related to} ~\ g,\\
                &\text{(Generalization)} \quad
                \;    \theta_{m,k,a}\mid \vx_{m,k},a&&= g(\vx_{m,k},a) +\delta_{m,k,a},\\
                & &&\quad \quad\quad
                \forall m\in[M],k\in[K_m],a\in\mathcal{A}_d, \\
                &\text{(Observation)} \quad
                \;\quad\quad \;   Y_{m,k,a,t}  &&=  \theta_{m,k,a_{m,k,t}} + \epsilon_{m,k,a_{m,k,t},t}, \\
                %& &&\quad \quad\quad \forall  m\in[M], k\in[K_m],\\
                &\text{(Reward)} \quad \quad\quad
                \quad\quad \quad \; R_{m,t} &&= \sum_{k\in[K_m]}Y_{m,k,a_{m,k,t},t},%\sum_{(k,a)\in A_{m,t}}Y_{m,k,a,t}.
            \end{alignedat}
        \end{equation} where $g(\vx_{m,k},a;\vgamma)$ takes different forms of working models including LR, GP, and NN.

As outlined in the main paper, the posterior updating process follows the bayesian updating rule
\begin{equation*}
    \mathds{P}(\vthe\mid \mH)\propto \mathds{P}(\vthe\mid \mH,g)\mathds{P}(g\mid \mH),
\end{equation*}
which naturally split the posterior derivation into two steps: 1) $\mathds{P}(g\mid\mH)$, and 2) $\mathds{P}(\vthe\mid\mH,g)$. 
\begin{comment}
With a slight abuse of notation, let $\vpsi$ be the general $d$-dimensional feature vector for a given campaign-adline-action tuple $(m, k, a)$. That is, $\vpsi_{m,k,a} := \phi(x_{m,k},a)$, and $\vpsi_{m} = \{\phi(x_{m,k},a)\}_{1\leq k\leq K, 1\leq a\leq N}$. As such, the three working models can be further summarized into the same framework as below:

\begin{equation}\label{General-version}
    \begin{alignedat}{2}
        &\text{(Prior)} \quad
        \quad\quad\quad \quad\quad \quad\quad  
        g(\cdot)&&\sim \mathcal{N}(\mu_{\vgamma}(\cdot), k_{\vgamma}(\cdot,\cdot'))\\
        %f&&\sim\mathcal{N}(\vmu_{\vgamma}, \Sigma_{\vgamma}) [\text{need to adjust}], \\
        &\text{(Generalization)} \quad
        \; \vthe_{m}\mid \vpsi_{m},g && = g(\vpsi_{m})+\vdelta_{m}, \forall m
    \end{alignedat}
\end{equation}

In LR, $\mu_{\vgamma}(x) = x'\vgamma$, $k_{\vgamma}(x,x') = x'\Sigma_{\vgamma} x$. In GP, $\mu_{\vgamma}(x)=\Phi(x)'\vgamma$ can take any specific function form of $x$ depending on the choice of $\Phi$, and $k_{\vgamma}(x,x') = \langle \Phi(x), \Phi(x')\rangle$ can take any kernel function such as linear kernel $k_{\vgamma}(x,x')=xx'$ and RBF kernel $k_{\vgamma}(x,x')= \exp\{-\|x-x'\|^2/(2\sigma^2)\}$. In NN, $\mu_{\vgamma}(x) = h(x;\vgamma)$ represents a fully-connected neural network with parameter $\vgamma$, and $k_{\vgamma}(x,x')$ represents the neural tangent kernel.
\end{comment}
In the subsequent sections, we will first derive the posterior distribution of $g$ given $\mH$ as a function form, and then derive the posterior distribution of $\vthe_m$ given $\mH$ and $g$. Since both LR and NN can be regarded as a special case of multivariate normal distribution given some transformed contextual information vector $x$, we will focus on the posterior derivation under Gaussian Process, and the expressions for LR and NN can be similarly derived with slight modifications, which are provided at the end of each subsection below.

\subsection{Posterior Distribution of \texorpdfstring{$g$}{g} Given \texorpdfstring{$\mH$}{H}}\label{step1_post}

In the Gaussian process, the Bayesian hierarchical model can be rewritten as
\begin{equation}
    \begin{alignedat}{2}
        &\text{(Prior)} \quad
        \quad\quad\quad \quad\quad \quad\quad  g&&\sim G P\left(\mu, \mathcal{K}\right), \\
        &\text{(Observation)} \quad
        \;\quad\quad \;   \vY_{1:H} && =g(\vPsi_{1:H})+\vdelta_{1:H}+\boldsymbol{\epsilon}_{1:H}, 
    \end{alignedat}
\end{equation}
where we define $\vdelta = (\vdelta_1^T,\dots,\vdelta_M^T)^T$ as the collection of the random effect vectors for all campaigns, $\vdelta_{1:H} = \vZ_{1:H}^T\vdelta\sim \normal(0,\Sigma_{1:H})$, and $\boldsymbol{\epsilon}_{1:H}\sim\normal(0,\sigma^2 I_{H})$. According to the definition above, $\Sigma_{1:H}= \vZ_{1:H}^{T}diag(\Cov, \cdots, \Cov)\vZ_{1:H}$.

Define $\boldsymbol{g}_{1:H} = g(\vPsi_{1:H})$ as the realization of Gaussian process $g$ under historical data $\vPsi_{1:H}$, and $\mathcal{K}_{1:H} = \mathcal{K}(\vPsi_{1:H},\vPsi_{1:H})$ as the covariance matrix for $\boldsymbol{g}_{1:H}$. The posterior of $g\mid \vY_{1:H}$ can be derived as
\begin{equation}\label{eq:GP1}
\begin{aligned}
    p(\boldsymbol{g}_{1:H}\mid \vY_{1:H}) &\propto p(\vY_{1:H}\mid \vPsi_{1:H},\boldsymbol{g}_{1:H})p(\boldsymbol{g}_{1:H}\mid \vPsi_{1:H})\\
    & \propto \exp\left( -\frac{1}{2} (\vY_{1:H}-\boldsymbol{g}_{1:H})^T (\sigma^2 I + \Sigma_{1:H})^{-1} (\vY_{1:H}-\boldsymbol{g}_{1:H})-\frac{1}{2}\boldsymbol{g}_{1:H}^T \mathcal{K}_{1:H}^{-1}\boldsymbol{g}_{1:H}\right)\sim \normal(\tilde\mu,\tilde{\Sigma})
\end{aligned}
\end{equation}
where 
\begin{equation}
    \begin{aligned}
    \tilde{\Sigma} &= \Big\{\mathcal{K}_{1:H}^{-1} + (\sigma^2 I + \Sigma_{1:H})^{-1}\Big\}^{-1}\\
    \tilde\mu &= (\sigma^2 I + \Sigma_{1:H})^{-1}\tilde{\Sigma} \vY_{1:H} = \big\{(\sigma^2 I + \Sigma_{1:H})+\mathcal{K}_{1:H}\big\}^{-1}\mathcal{K}_{1:H} \vY_{1:H}.
    \end{aligned}
\end{equation}

When a new sample $x^*$ comes in, the posterior distribution of $g^*\mid x^*,\mathcal{H}$ is given by
\begin{equation}\label{eq:GP2}
    p(g^*\mid x^*,\mathcal{H}) =\int p(g^*,\boldsymbol{g}_{1:H}\mid x^*,\mathcal{H}) d \boldsymbol{g}_{1:H} = \int p(g^*\mid \boldsymbol{g}_{1:H},x^*,\mathcal{H}) p(\boldsymbol{g}_{1:H}\mid x^*,\mathcal{H}) d\boldsymbol{g}_{1:H}.
\end{equation}

\begin{comment}
For the ease of presentation, we define 
\begin{equation}
    \begin{aligned}
    \boldsymbol{a} = 
    \end{aligned}
\end{equation}   
\end{comment}

Since $p(g^*\mid \boldsymbol{g}_{1:H}) \sim \normal \big(\mathcal{K}(x^*,\vPsi_{1:H})\mathcal{K}_{1:H} \boldsymbol{g}_{1:H}, \mathcal{K}(x^*,x^*)- k(x^*,\vPsi_{1:H})\mathcal{K}_{1:H} \mathcal{K}(\vPsi_{1:H},x^*)\big)$, we can combine it with \eqref{eq:GP1} and \eqref{eq:GP2} to obtain the posterior mean and variance for $ p(g^*\mid x^*,\mathcal{H})$.

After some tedious but conceptually straightforward manipulations, the posterior mean and variance of $g\mid \mathcal{H}$ can be derived as
\begin{equation}\label{eq:fstar_post}
\begin{aligned}
    \mu_{\text{post}}(x) &=\mu(x) + \mathcal{K}(x,\vPsi_{1:H})[\mathcal{K}(\vPsi_{1:H},\vPsi_{1:H})+\sigma^2 I + \Sigma_{1:H}]^{-1} (\vY_{1:H}-\mu(\vPsi_{1:H}))\\
    \mathcal{K}_{\text{post}}(x,x') &= \mathcal{K}(x,x') - \mathcal{K}(x,\vPsi_{1:H})[\mathcal{K}(\vPsi_{1:H},\vPsi_{1:H})+\sigma^2 I + \Sigma_{1:H}]^{-1} \mathcal{K}(\vPsi_{1:H},x')
\end{aligned}
\end{equation}
with $\Sigma_{1:H}= \vZ_{1:H}^{T}diag(\Cov, \cdots, \Cov)\vZ_{1:H}$.

In LR and NN, since the prior was imposed on a finite-dimensional parameter $\vgamma$, one can similarly derive the posterior of $\vgamma\mid \mH$ as below:
\begin{align*}
    &\mathbb{E}(\vgamma\mid \mH) = \text{Cov}(\vgamma\mid \mH)\{\vPsi_{1:H}(\Sigma_{1:H}+\sigma^{2}\vI)^{-1}\vY_{1:H} + \Sigma_{\vgamma}^{-1}\vmu_{\vgamma}\}\\%\vmu_{\vgamma} + {\Cov}_{\vgamma}\vPsi_{1:H}(\vZ_{1:H}^{T}diag(\Cov, \cdots, \Cov)\vZ_{1:H}+\sigma^{2}\vI+\vPsi_{1:H}^T{\Cov}_{\vgamma}\vPsi_{1:H})^{-1}(\vY_{1:H}-\vPsi_{1:H}^T\vmu_{\vgamma});\\
    &\text{Cov}(\vgamma\mid \mH) = \left(\vPsi_{1:H}(\Sigma_{1:H}+\sigma^{2}\vI)^{-1}\vPsi_{1:H}^T+{\Cov}_{\vgamma}^{-1}\right)^{-1}\\
    & \qquad\qquad\quad = \Sigma_{\vgamma} - \Sigma_{\vgamma}\vPsi_{1:H}[\vPsi_{1:H}'\Sigma_{\vgamma}\vPsi_{1:H}+\sigma^2 I + \Sigma_{1:H}]^{-1} \vPsi_{1:H}'\Sigma_{\vgamma} ,%{\Cov}_{\vgamma}-{\Cov}_{\vgamma}\vPsi_{1:H}(\vZ_{1:H}^{T}diag(\Cov, \cdots, \Cov)\vZ_{1:H}+\sigma^{2}\vI+\vPsi_{1:H}^T{\Sigma}_{\vgamma}\vPsi_{1:H})^{-1}\vPsi_{1:H}^T{\Sigma}_{\vgamma}.
\end{align*}
where the second equation in $\text{Cov}(\vgamma\mid \mH)$ is a direct application of the Woodbury matrix identity.

In both LR and NN, $g(x)$ shares a similar linear structure defined by $g(x) = \phi(x)^T\vgamma$, where $\phi(x)$ denoting different feature information representations. Specifically, for LR, $\phi(x)$ can be as simple as $x$; for NN,  $\vgamma=\{\text{vec}(W_1),\cdots, \text{vec}(W_L)\}$ represents the collection of parameters of the neural network, $L$ is the number of layers, and $g$ is a fully connected neural network of depth $L\geq 2$. $\phi(x)$ is the gradient of the neural network.

As such, the posterior mean and variance of $g(x)\mid \mH$ can be obtained by directly multiplying $\phi(x)$ on the posterior of $\vgamma\mid \mH$:
\begin{equation}
\begin{aligned}
    \mathbb{E}(g(x)\mid \mH) &=\phi(x)'\vgamma + x'\Sigma_{\vgamma}\vPsi_{1:H} [\vPsi_{1:H}'\Sigma_{\vgamma}\vPsi_{1:H}+\sigma^2 I + \Sigma_{1:H}]^{-1} (\vY_{1:H}-\vPsi_{1:H}'\vgamma)\\
    \text{Cov}(g(x)\mid \mH) &= x'\Sigma_{\vgamma} x - x'\Sigma_{\vgamma}\vPsi_{1:H}[\vPsi_{1:H}'\Sigma_{\vgamma}\vPsi_{1:H}+\sigma^2 I + \Sigma_{1:H}]^{-1} \vPsi_{1:H}'\Sigma_{\vgamma} x,
\end{aligned}
\end{equation}
which exactly aligns with the general posterior formulation we derived for GP in Equation \eqref{eq:fstar_post}.

\subsection{Posterior Distribution of \texorpdfstring{$\vthe$}{theta} Given \texorpdfstring{$\mH$}{H} and \texorpdfstring{$g$}{g}} \label{step2_post}

According to the observation layer in (\ref{appendix:model}), the posterior distribution of $\vY_{1:H}\mid \vPsi_{1:H},\vthe$ is given by
\begin{align*}
    \vY_{1:H}\mid \vPsi_{1:H},\vthe \sim \normal(\vZ_{1:H}^{T}\vthe,\sigma^{2}\vI_{KH}).
\end{align*}
Then, the posterior distribution of $\vthe$ given $\mH$ and $\vgamma$ is
\begin{align*}
    & \quad \mathds{P}(\vthe\mid \vY_{1:H},g) \\
    &\propto \mathds{P}(\vY_{1:H}\mid \vthe)\mathds{P}(\vthe\mid g)\\
    &\propto exp\Big(-\frac{1}{2}\sigma^{-2}(\vY_{1:H}-\vZ_{1:H}^{T}\vthe)^{T}(\vY_{1:H}-\vZ_{1:H}^{T}\vthe)\Big) exp\Big(-\frac{1}{2}(\vthe-g(\vPsi))^{T}diag(\Cov^{-1},\cdots,\Cov^{-1})(\vthe-g(\vPsi))\Big)\\
    &\propto exp\Big(-\frac{1}{2}\vthe^{T}\underbrace{(\sigma^{-2}\vZ_{1:H}\vZ_{1:H}^{T}+diag(\Cov^{-1},\cdots, \Cov^{-1}))}_{\Cov_{**}^{-1}}\vthe+\vthe^{T}\{\sigma^{-2}\vZ_{1:H}\vY_{1:H}+diag(\Cov^{-1},\cdots, \Cov^{-1})g(\vPsi)\}\Big)\\
    &\sim \normal(\underbrace{\Cov_{**}\{\sigma^{-2}\vZ_{1:H}\vY_{1:H}+diag(\Cov^{-1},\cdots, \Cov^{-1})g(\vPsi)\}}_{\vmu_{**}},\Cov_{**}).
\end{align*}
%Using the Woodbury matrix identity, we have
%\begin{align*}
%    \vmu_{**} = \vX^T\vgamma + diag(\Cov,\cdots, \Cov)\vZ_{1:H}\big[\sigma^{2}\vI_{KH}+\vZ_{1:H}^{T}diag(\Cov,\cdots, \Cov)\vZ_{1:H}\big]^{-1}(\vY_{1:H}-\vPsi_{1:H}^T\vgamma).
%\end{align*}
Let $C_{m,k,n}$ be the number of observations in $\mH$ that correspond to base arm $(m,k,n)$. We have that
\begin{align*}
    \sigma^{-2}\vZ_{1:H}\vZ_{1:H}^{T}+diag(\Cov^{-1},\cdots, \Cov^{-1})
    &= \sigma^{-2}diag(C_{1,1,1},\cdots,C_{M,K,N})+diag(\Cov^{-1},\cdots, \Cov^{-1})\\
    &=\begin{bmatrix}
    \Cov^{-1}+\sigma^{-2}diag(C_{1,1,1},\cdots, C_{1,K,N}) & & \\
    & \ddots & \\
    & & \Cov^{-1}+\sigma^{-2}diag(C_{M,1,1},\cdots, C_{M,K,N})
  \end{bmatrix}.
\end{align*}
Therefore, for each campaign $m \in [M]$, the posterior of $\vthe_m$ follows a normal distribution with mean and variance as:
\begin{align*}
    &\mathbb{E}(\vthe_m\mid \mH, g) = Cov(\vthe_m\mid \mH, g)
    \left[\Cov^{-1}g(\vPsi_m) + \sigma^{-2}\vZ_{1:H,m}\vY_{1:H}\right],\\
    &Cov(\vthe_m\mid \mH, g) = \left(\Cov^{-1}+\sigma^{-2}diag(C_{m,1,1},\cdots, C_{m,K,N})\right)^{-1},
\end{align*} where $\vZ_{1:H,m}$ is a subset of $\vZ_{1:H}$ that contains all rows corresponding to ad lines within campaign $m$.It's noteworthy that regardless of the working model from which $g$ is sampled, the posterior formula for $\vthe_m\mid \mH, g$ remains identical for LR, GP, and NN.

\subsection{Batch Update and Memory Check}\label{appendix:batch_memory}
In this section, we outline two strategies to enhance the bandit updating process. At each round $t$, our primary algorithm comprises two steps: 1) updating the posterior of $g$, and 2) updating the posterior mean $\theta_{m,k,a}$. In GP, the posterior formulations for $g|\mH$ involve the inverse of a large matrix whose dimension increases with the number of observed samples ($KH$). While in LR and NN, the Woodbury Identity matrix can be employed to expedite the inverse calculation, this method is not applicable in GP.

To improve computational efficiency, it is often unnecessary to update both 1) and 2) whenever a single data point is introduced, particularly in Gaussian Process where computational complexity poses a common challenge in the posterior updating process. Recent literature has seen a surge in papers addressing the acceleration of GP-based Bayesian regression \cite{wilson2020efficiently, vakili2021scalable}. In this study, we integrate two fundamental and highly effective approaches -- batch update and memory check -- that demonstrate robust performance in both simulation and real data analysis.

\begin{figure}[tbh]
    \centering
    \includegraphics[width=0.9\linewidth]{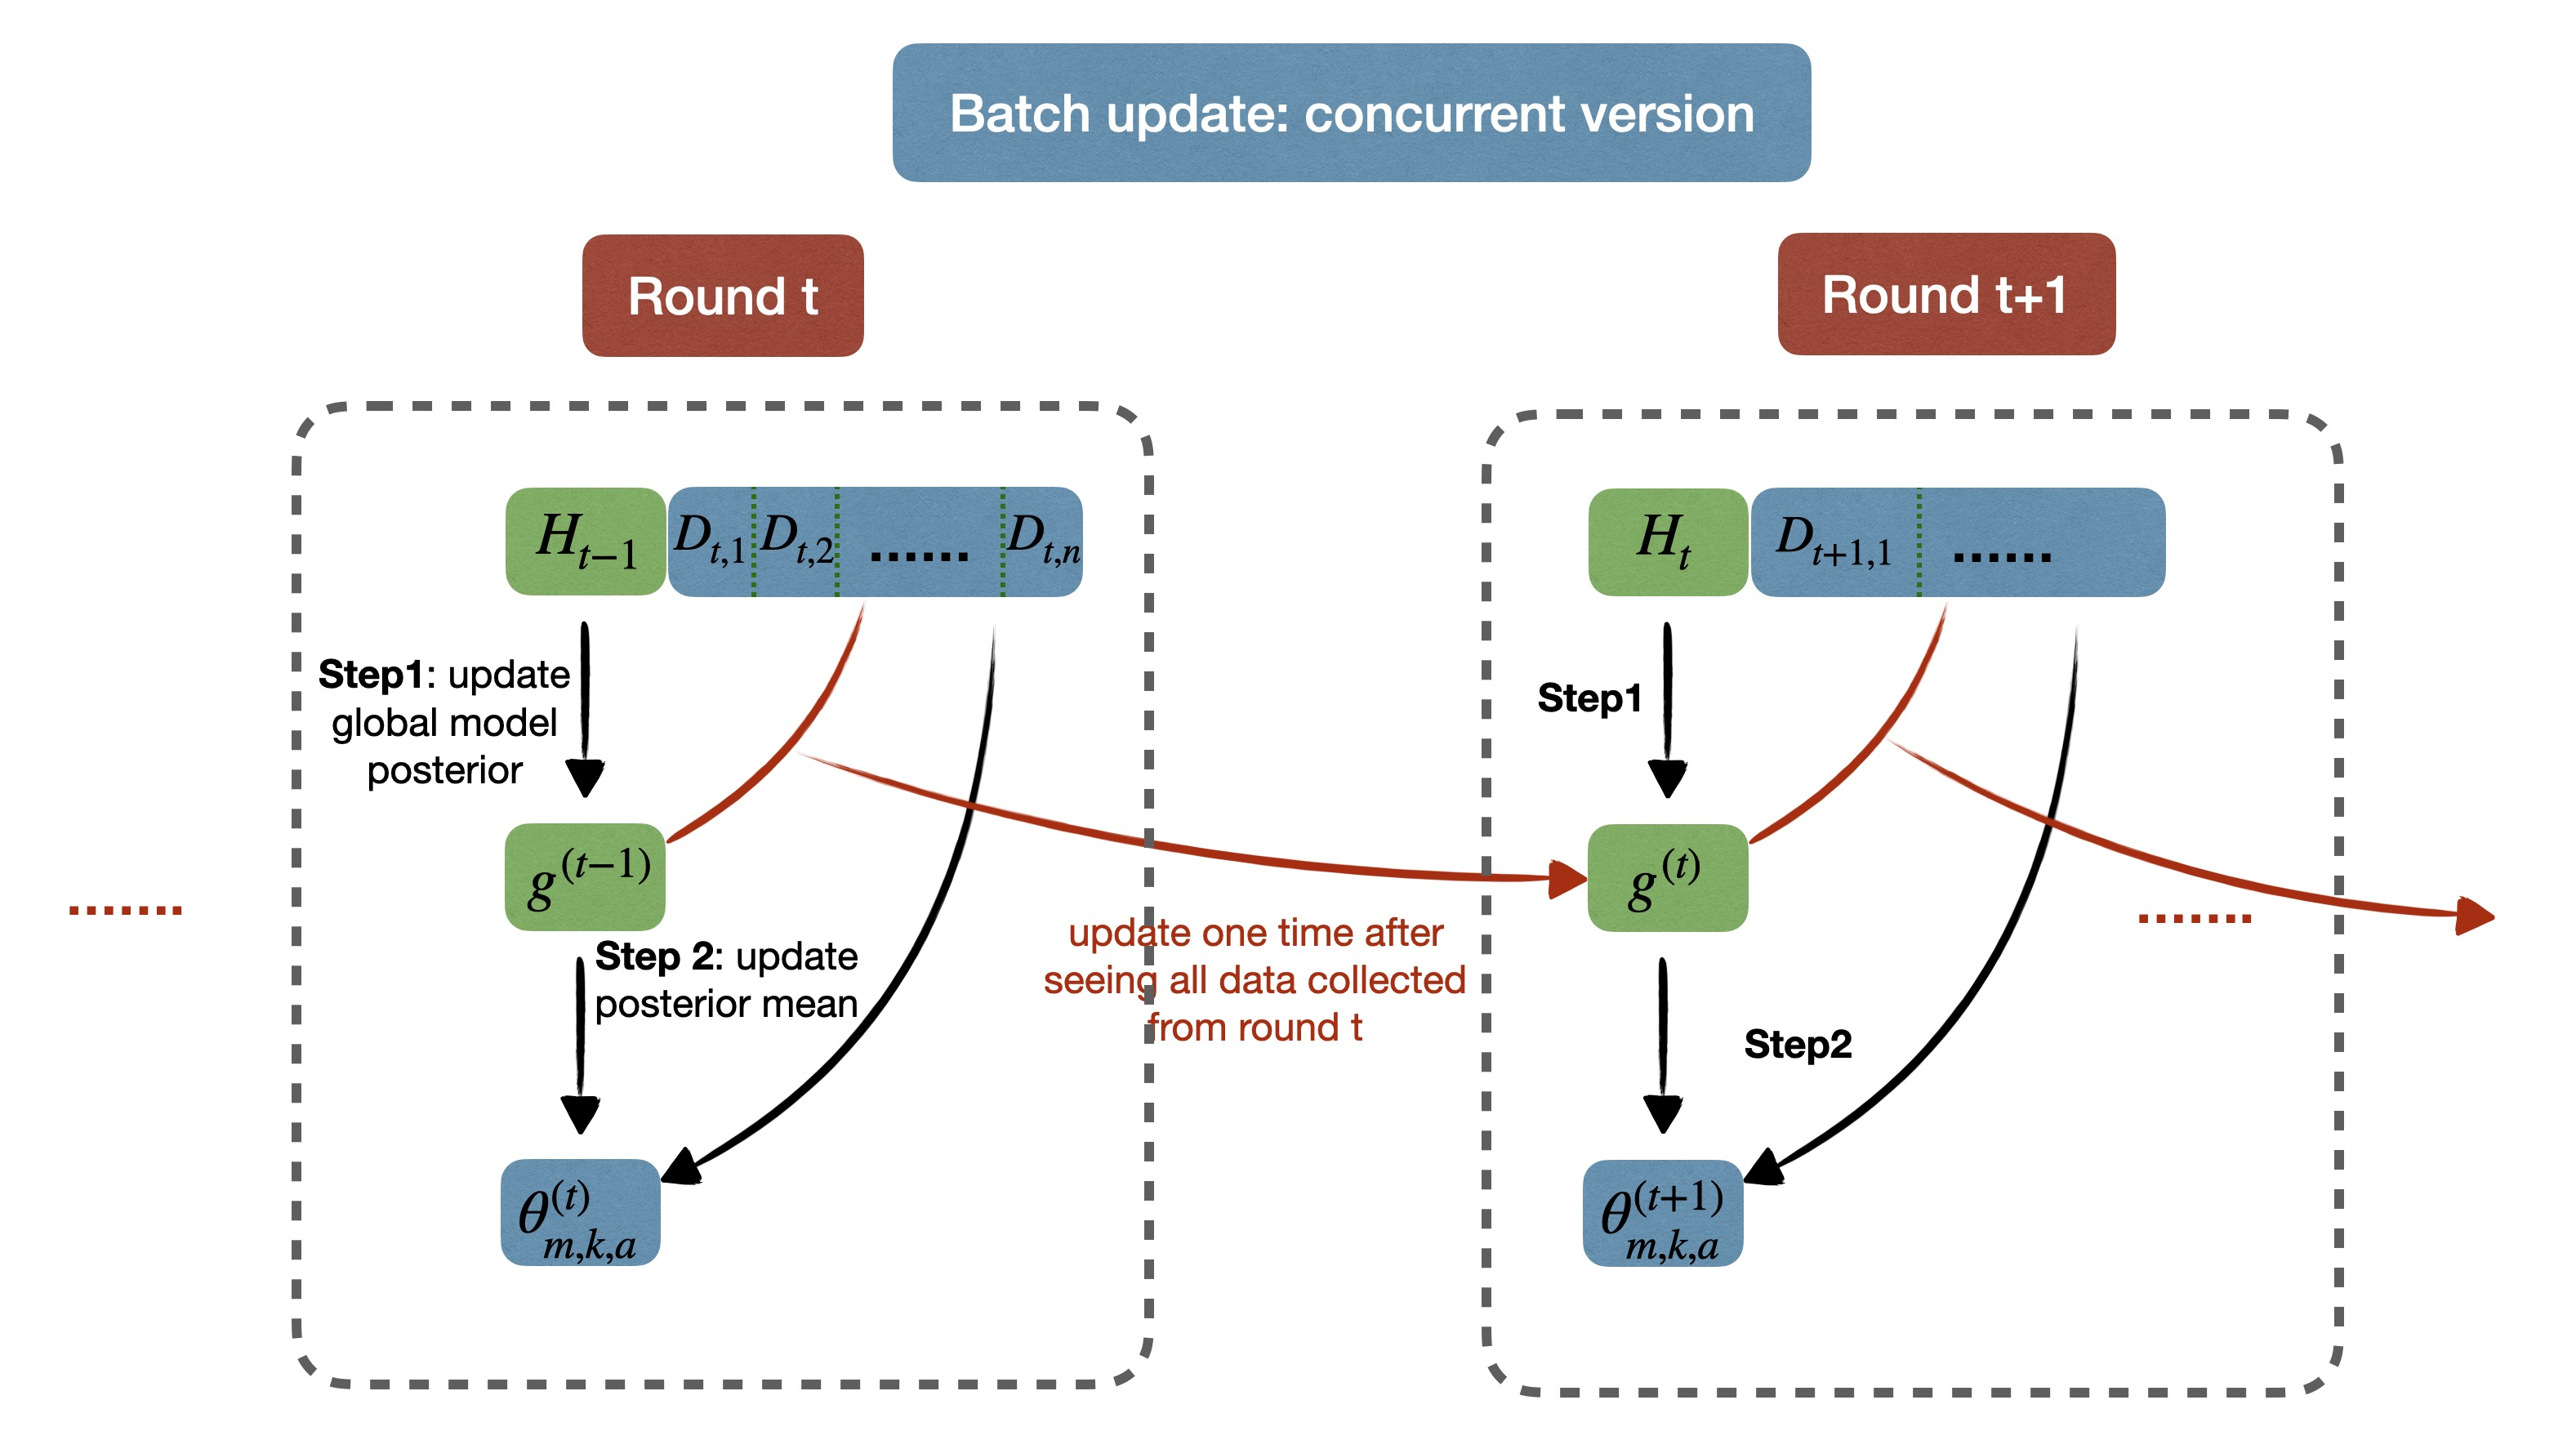}
    \caption{concurrent only}
    \label{fig:batch1}
\end{figure}

\begin{figure}[tbh]
    \centering
    \includegraphics[width=0.9\linewidth]{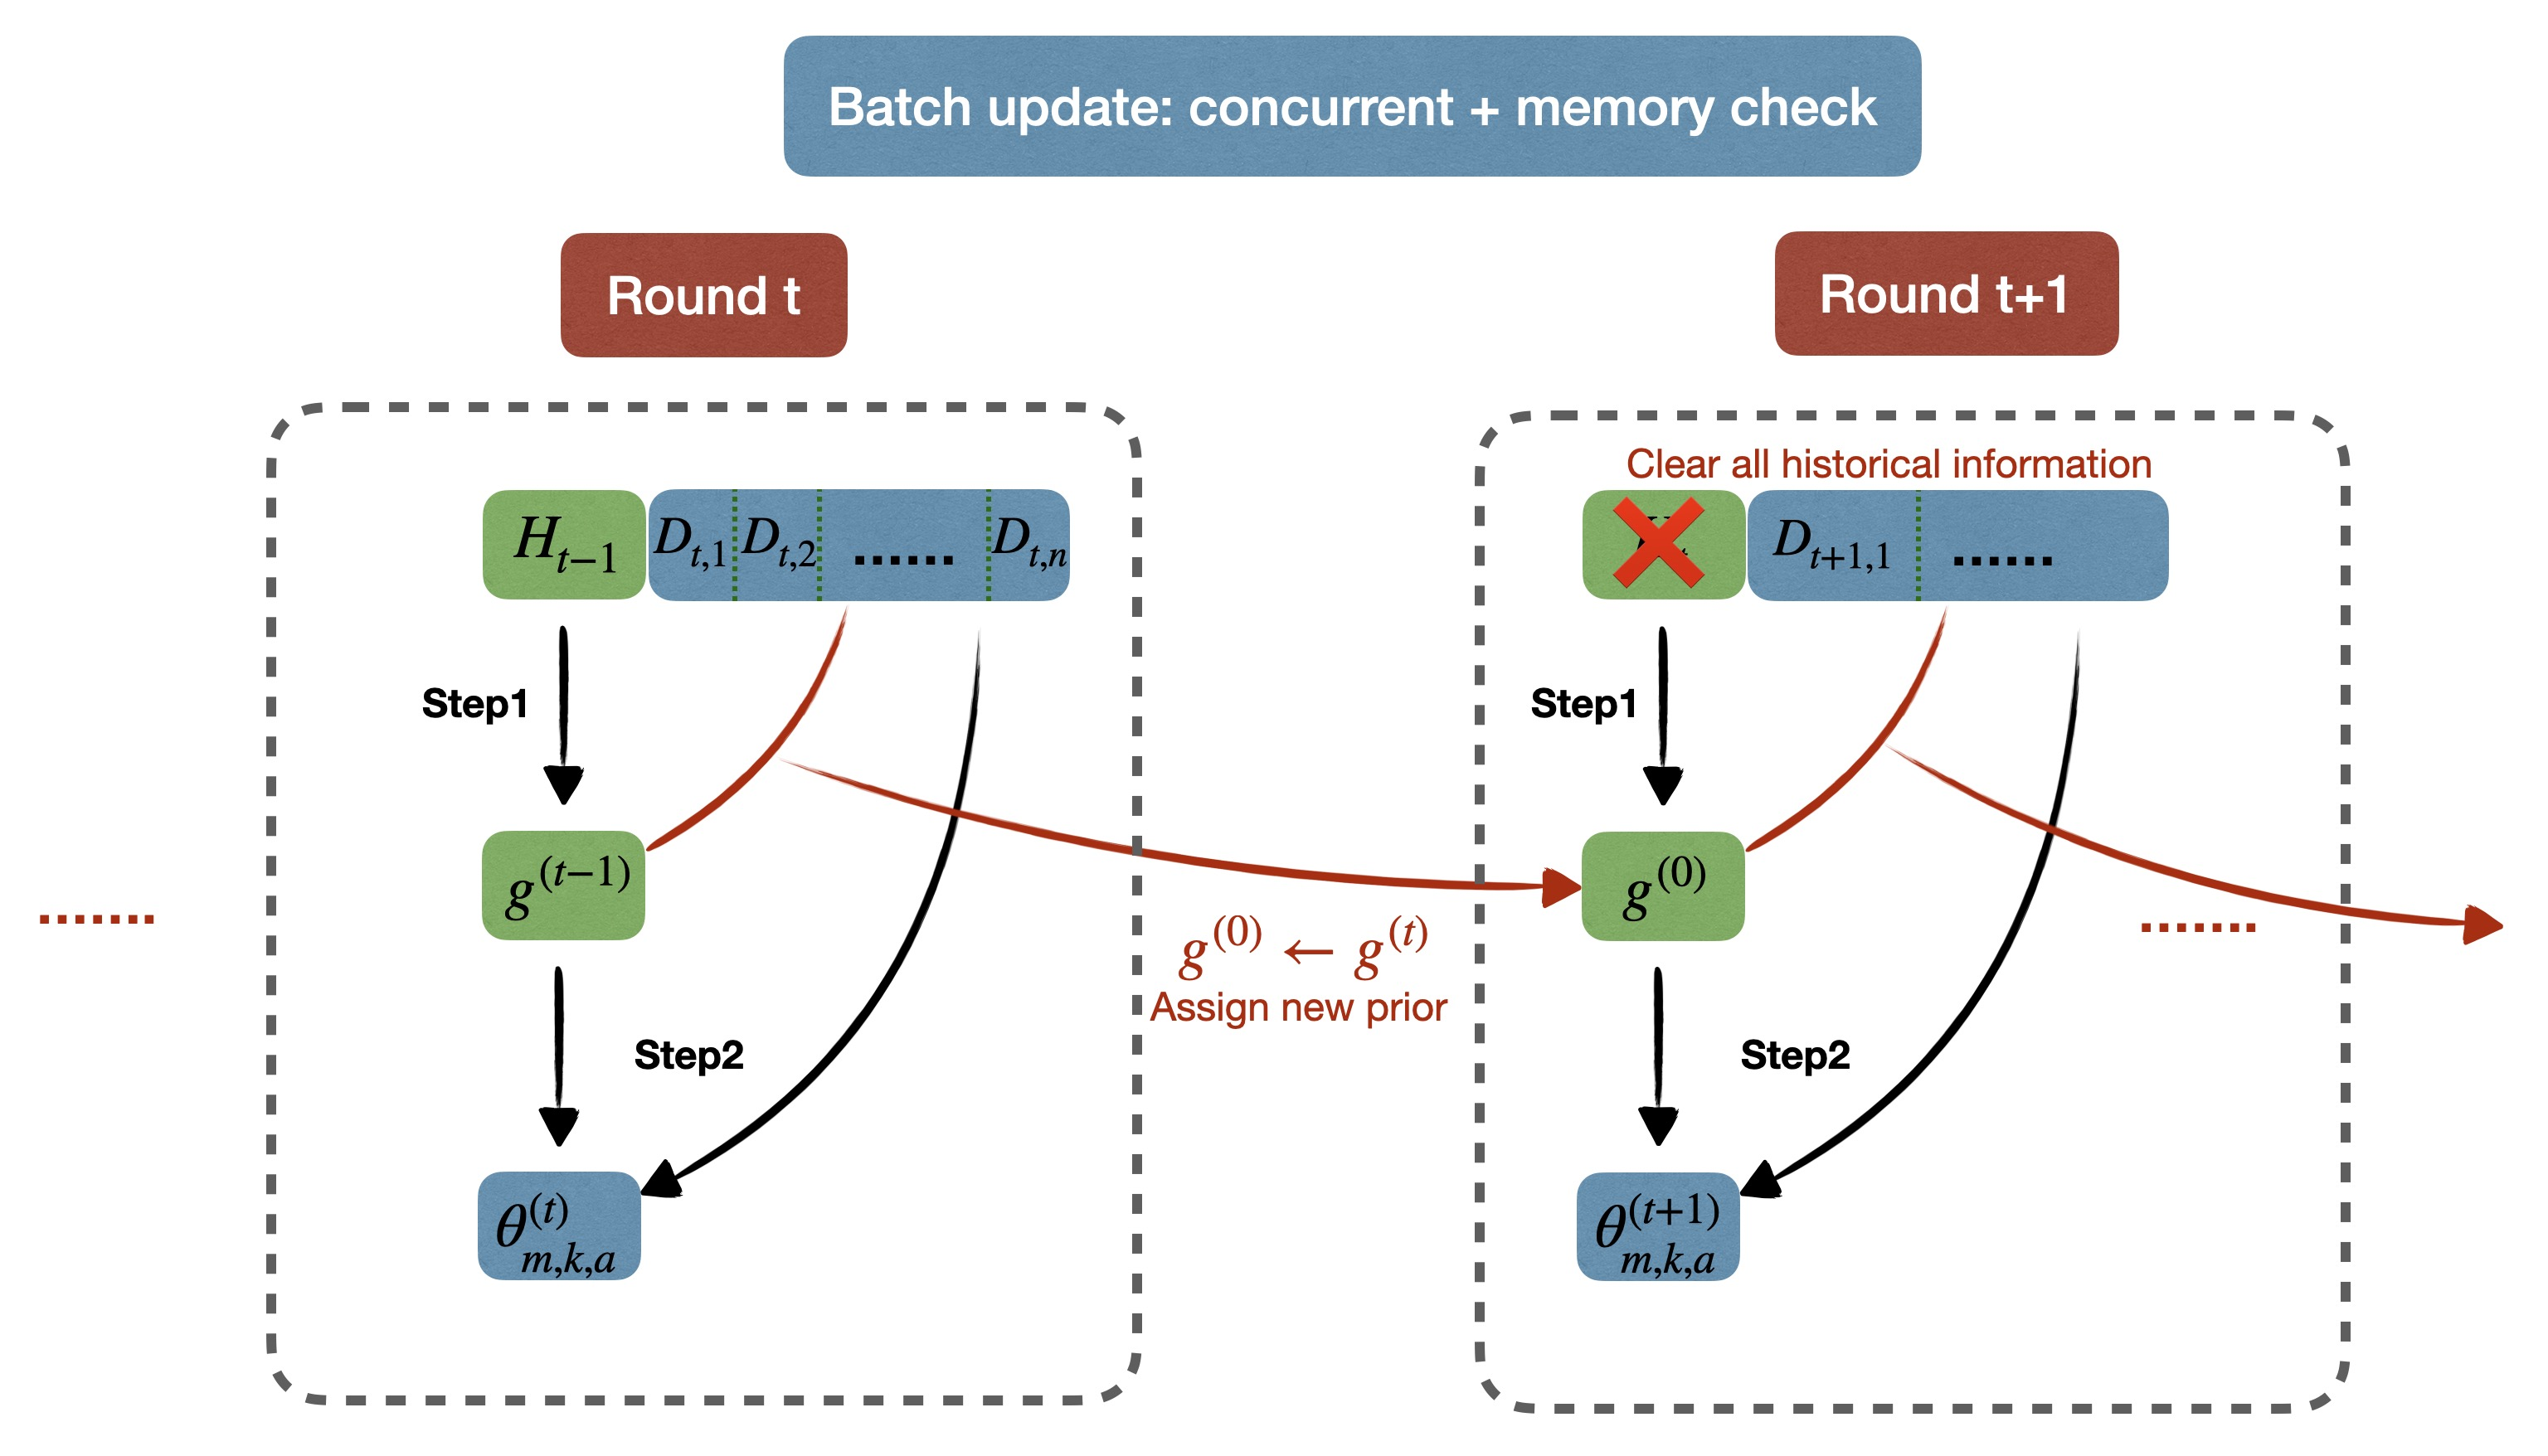}
    \caption{concurrent + memory check}
    \label{fig:batch2}
\end{figure}

\begin{enumerate}
    \item \textbf{Batch Update}: In our problem setup, each day involves the observation of multiple data points coming from various concurrent campaigns. Rather than updating the posterior of both 1) $f$ and 2) $\theta_{m,k,a}$ for every individual data point, we implemented a batch update procedure outlined in Figure \ref{fig:batch1}. Let $H_t = \{D_{t,1},\dots,D_{t,n}\}$ represent the collection of all data points observed at round $t$. At the beginning of each day, $H_{t-1}$ is utilized to update the posterior of 1), denoted as $f^{(t-1)}$. Subsequently, upon gathering all data points on day $t$, $H_t$ is employed to update the posterior of 2), denoted as $\theta_{m,k,a}^{(t)}$. The data in $H_t$ is then used for the posterior update of $f^{(t)}$ in round $t+1$.
    \item \textbf{Memory Check (specifically for GP)}: To further accelerate the posterior updating process, we introduced a memory check procedure (Figure \ref{fig:batch2}) within the GP framework, based on the batch update process in Step 1. The concept is straightforward: just as in real-world scenarios where very old historical data requires periodic cleanup, in GP, we incorporate a memory check threshold into the algorithm. Upon reaching this threshold, the matrix that needs inversion triggers the storage of posterior information for $f^{(t)}$ in a $M\times K\times N$ dimensional matrix. Simultaneously, all historical data up to $H_t$ is deleted. In the subsequent round $t+1$, $f^{(t)}$ is treated as a new prior $f^{(0)}$, and the original updating process persists until the next memory check threshold is reached.
 \end{enumerate}

Based on our empirical study, both of these approaches significantly reduce the running time with negligible computational error in terms of average regret. Therefore, we only present the results with batch update and memory check in our main paper.

\begin{comment}
\subsubsection{Other Graphs}

\begin{figure}[tbh]
    \centering
    \includegraphics[width=0.9\linewidth]{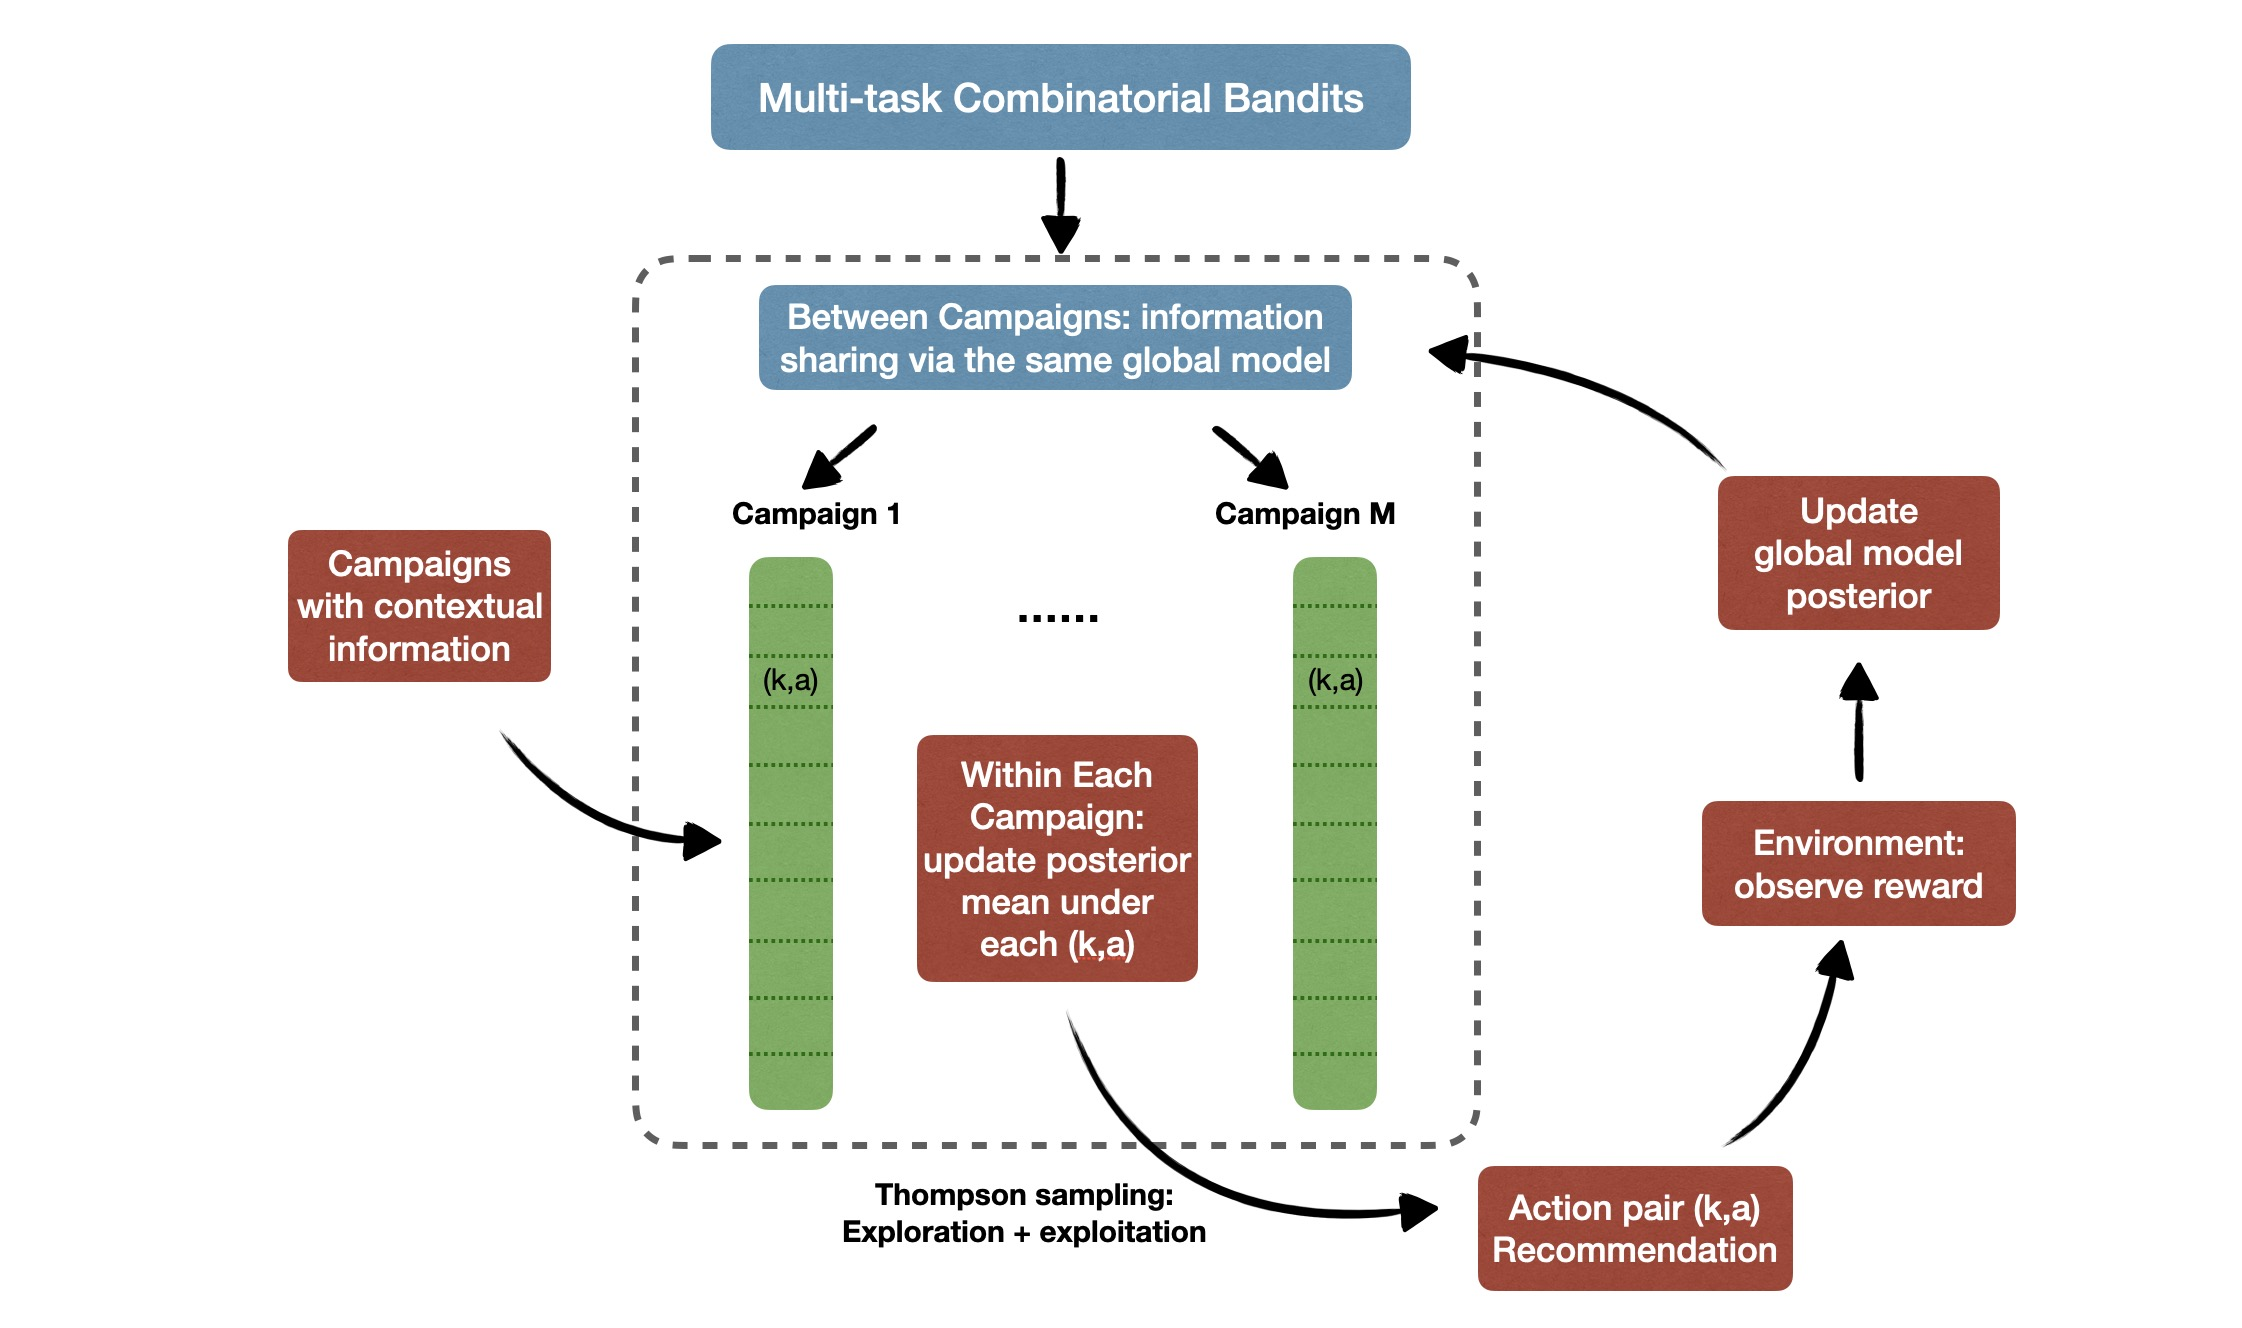}
    \caption{flowchart}
    \label{fig:flow}
\end{figure}
\end{comment}
