# Supplementary material for: Multi-Task Combinatorial Bandits for Budget Allocation
Source: arXiv:2409.00561 source file (2024-08-31)
Supplement: Supplementary file 2 [file 8.Appendix3.tex]

\section{Additional Experiment Results}\label{addtional exp}
In this section, we present additional results for the MCMAB's performance under various settings of $(M, K, N, d, \sigma_\epsilon)$. Specifically, Figures \ref{fig:LMM_M}-\ref{fig:LMM_sigma} examine MCMAB's behavior in a concurrent linear environment, using LR as the working model. To minimize computational costs, we set a baseline hyper-parameter configuration as $\Cov = \sigma_m^2\boldsymbol{I} = .75^2\boldsymbol{I}$, $M = 50$, $K = 5$, $N = 50$, $\sigma_\epsilon = 1$, and $d_m = d_k = 3$. All findings are averaged over 100 random seeds. Overall, MCMAB consistently outperforms other baseline methods, achieving lower regrets that gradually approach the performance of the oracle-TS. Our results can be summarized as follows:
\begin{itemize}
    \item With an increase in $M$ (Figure \ref{fig:LMM_M}), MCMAB effectively learns the task distribution, benefiting from the availability of more diverse metadata, especially in the initial stages.

    \item As $K$ increases (Figure \ref{fig:LMM_K}), MCMAB effectively learns the task distribution more quickly, despite the expected rise in optimization and learning complexity. This is attributed to the greater availability of data for environmental estimation and the robust performance of the efficient dynamic programming algorithm.

    \item With a higher $N$ (Figure \ref{fig:LMM_N}), although the learning challenge intensifies for all algorithms, MCMAB maintains lower regret levels.

    \item An increase in $d_m/d_k$ (Figure \ref{fig:LMM_d}) adds complexity to the learning process. Nevertheless, MCMAB begins to show superior performance, even with a limited time horizon of $T=20$.

    \item As $\sigma_\epsilon$ rises (Figure \ref{fig:LMM_sigma}), the learning task complexity increases, yet MCMAB still exhibits a clear advantage.

\end{itemize}

\begin{figure}[h]
    \centering
    \includegraphics[width = .75\linewidth]{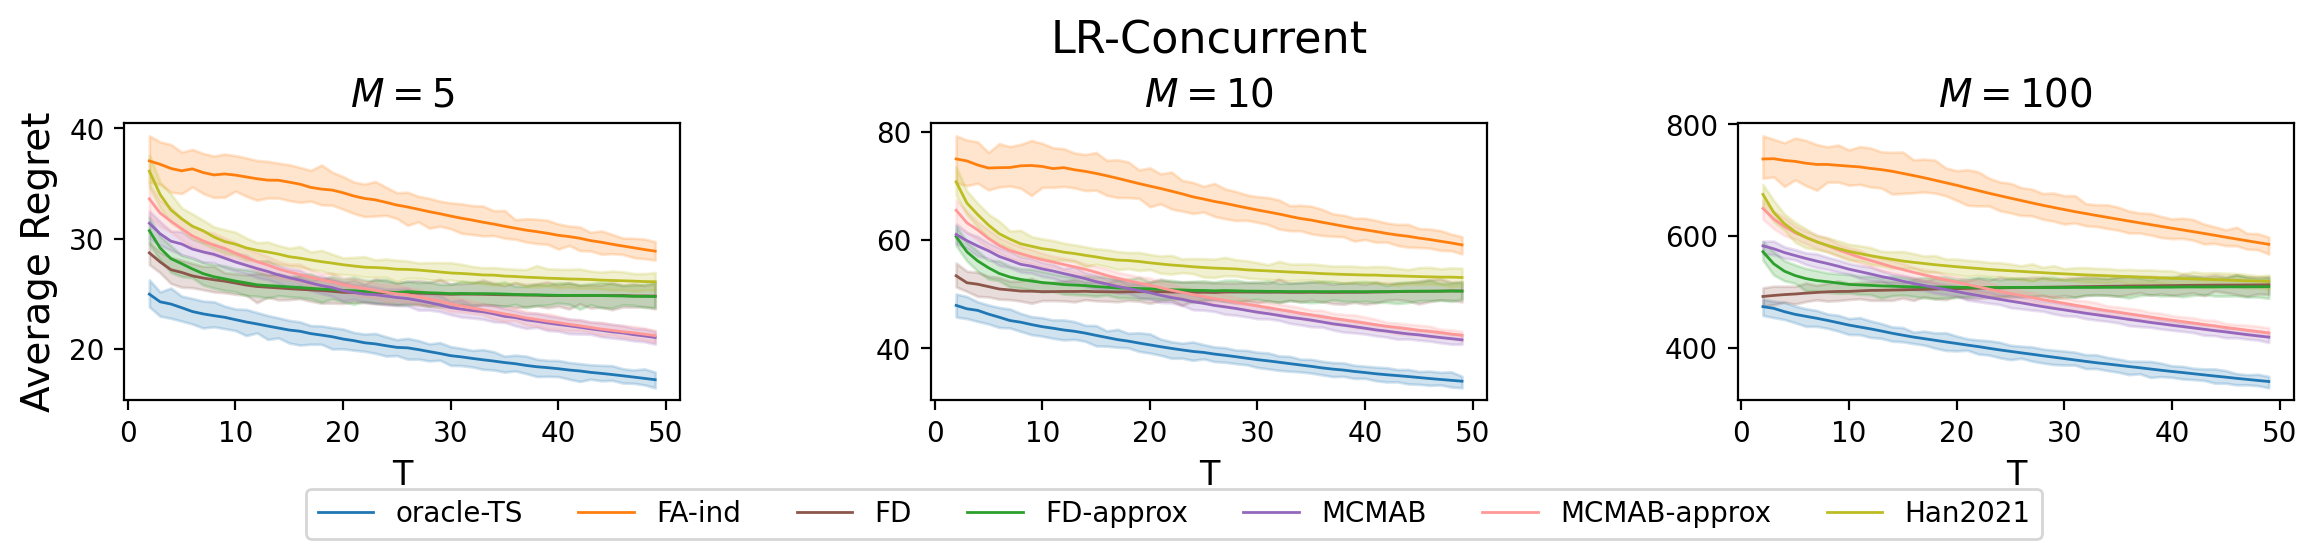}
    \caption{Simulation results for the concurrent linear environment setting with different $M$ specifications. Shaded areas indicate the 95\% confidence interval.}
    \label{fig:LMM_M}
\end{figure}

\begin{figure}[h]
    \centering
    \includegraphics[width = .75\linewidth]{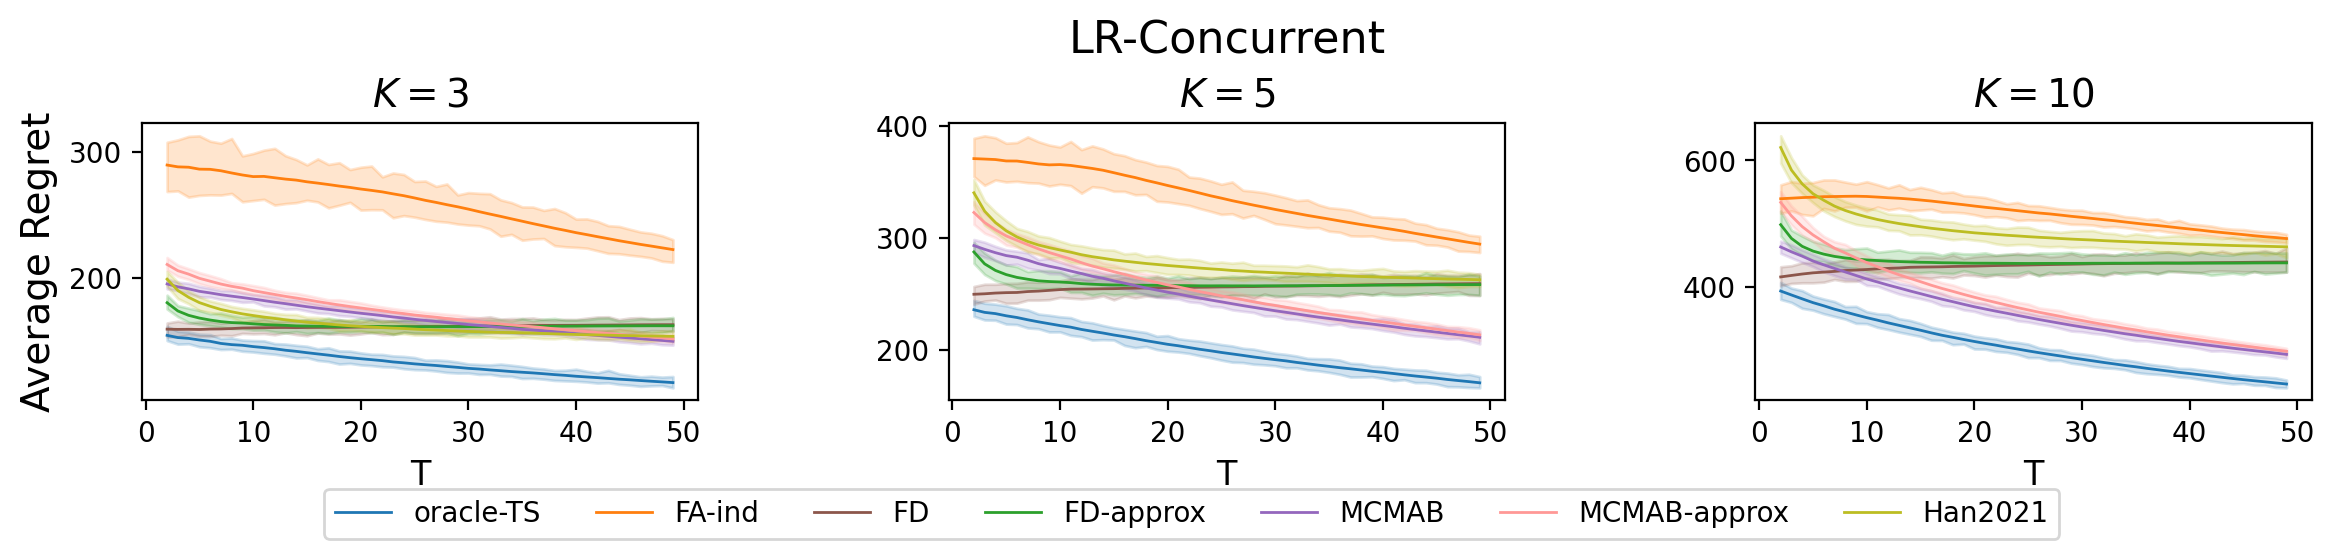}
    \caption{Simulation results for the concurrent linear environment setting with different $K$ specifications. Shaded areas indicate the 95\% confidence interval.}
    \label{fig:LMM_K}
\end{figure}

\begin{figure}[h]
    \centering
    \includegraphics[width = .75\linewidth]{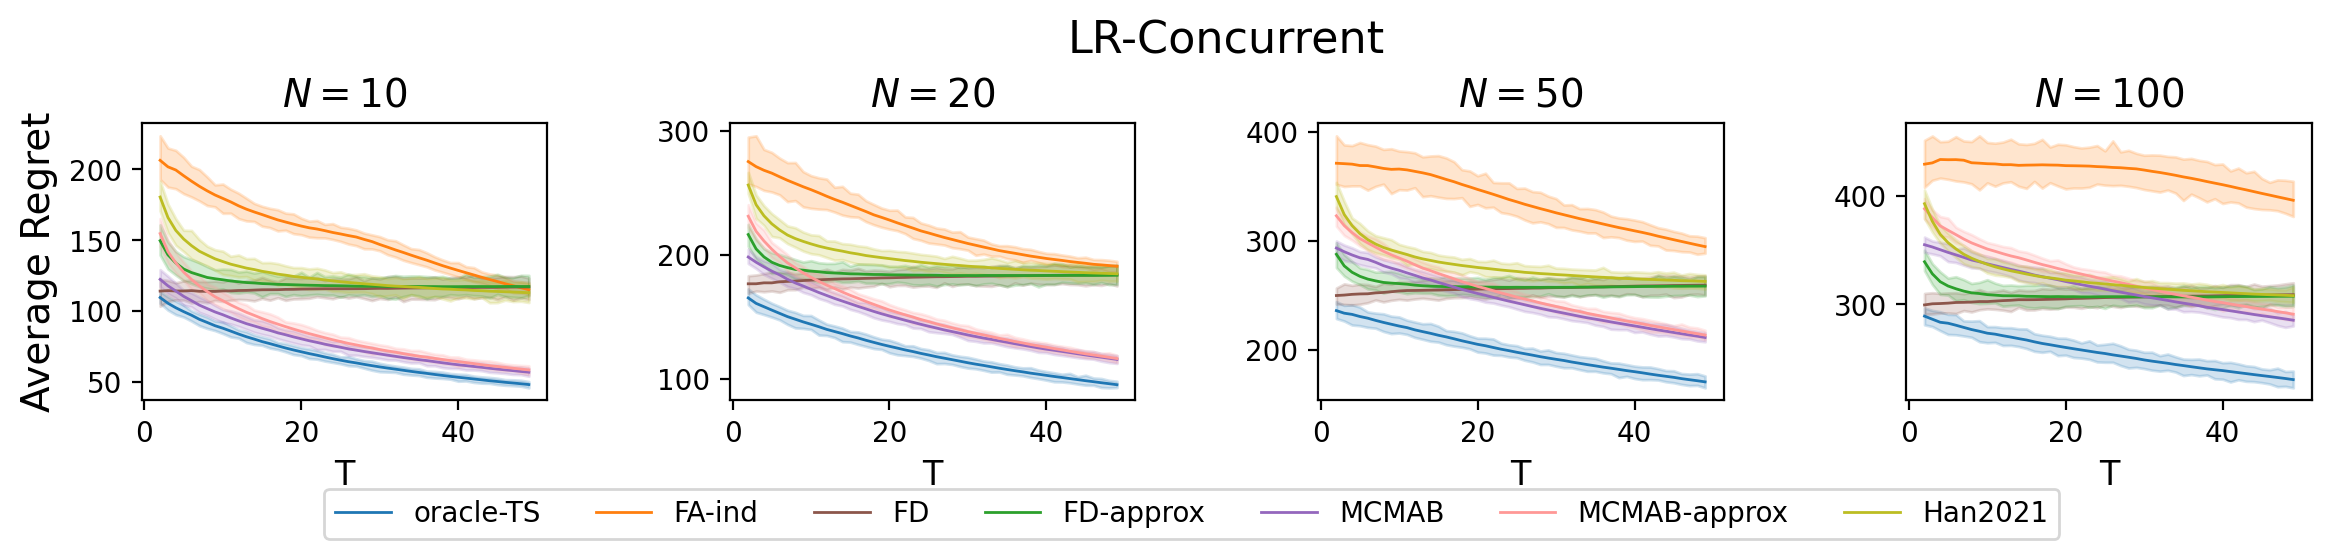}
    \caption{Simulation results for the concurrent linear environment setting with different $N$ specifications. Shaded areas indicate the 95\% confidence interval.}
    \label{fig:LMM_N}
\end{figure}

\begin{figure}[h]
    \centering
    \includegraphics[width = .75\linewidth]{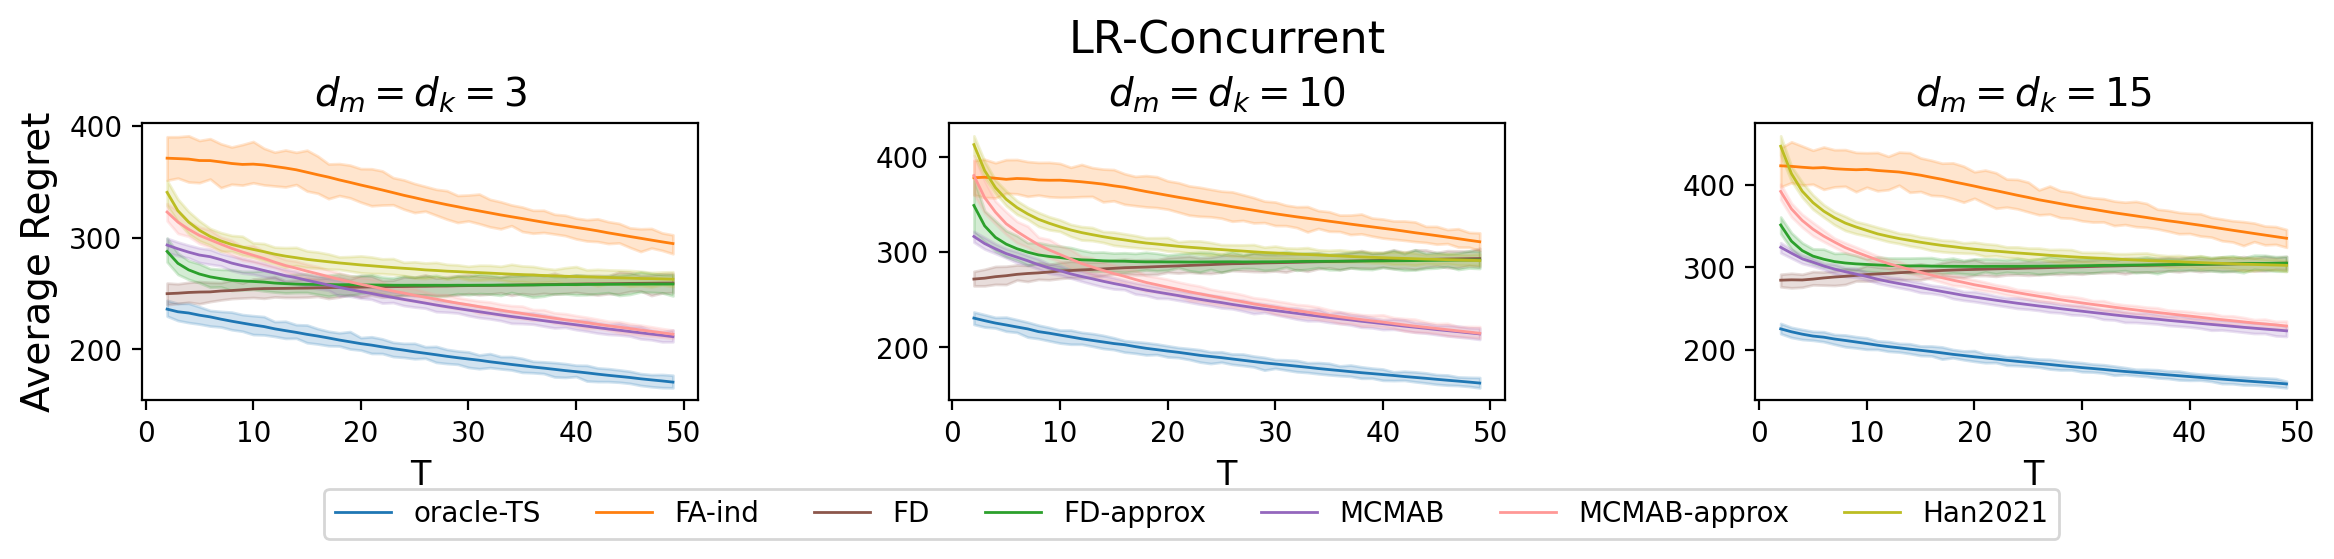}
    \caption{Simulation results for the concurrent linear environment setting with different $d$ specifications. Shaded areas indicate the 95\% confidence interval.}
    \label{fig:LMM_d}
\end{figure}

\begin{figure}[h]
    \centering
    \includegraphics[width = .75\linewidth]{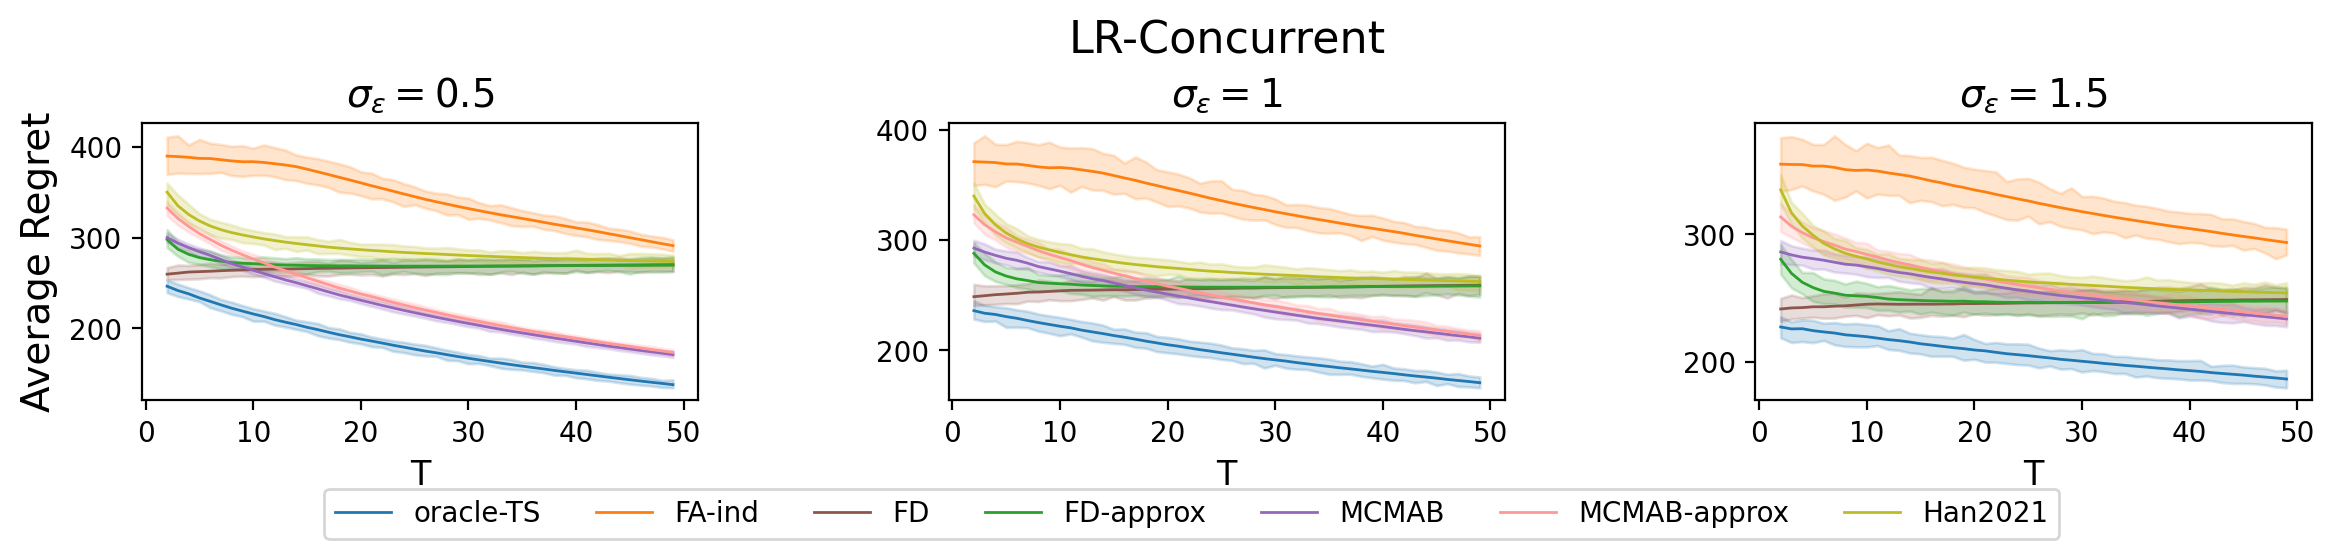}
    \caption{Simulation results for the concurrent linear environment setting with different $\sigma_\epsilon$ specifications. Shaded areas indicate the 95\% confidence interval.}
    \label{fig:LMM_sigma}
\end{figure}

Additionally, we explore the performance of MCMAB with GP and NN as working models in the concurrent nonlinear environments with different specifications of $d_m/d_k$ in Figure \ref{fig:GP_d} and Figure \ref{fig:NN_d}, respectively. Similar to what we observed in Figure \ref{fig:LMM_d}, as $d_m/d_k$ increases, the learning process gets more complicated, but MCMAB still demonstrates better performance than other baseline algorithms.

\begin{figure}[h]
    \centering
    \includegraphics[width = .75\linewidth]{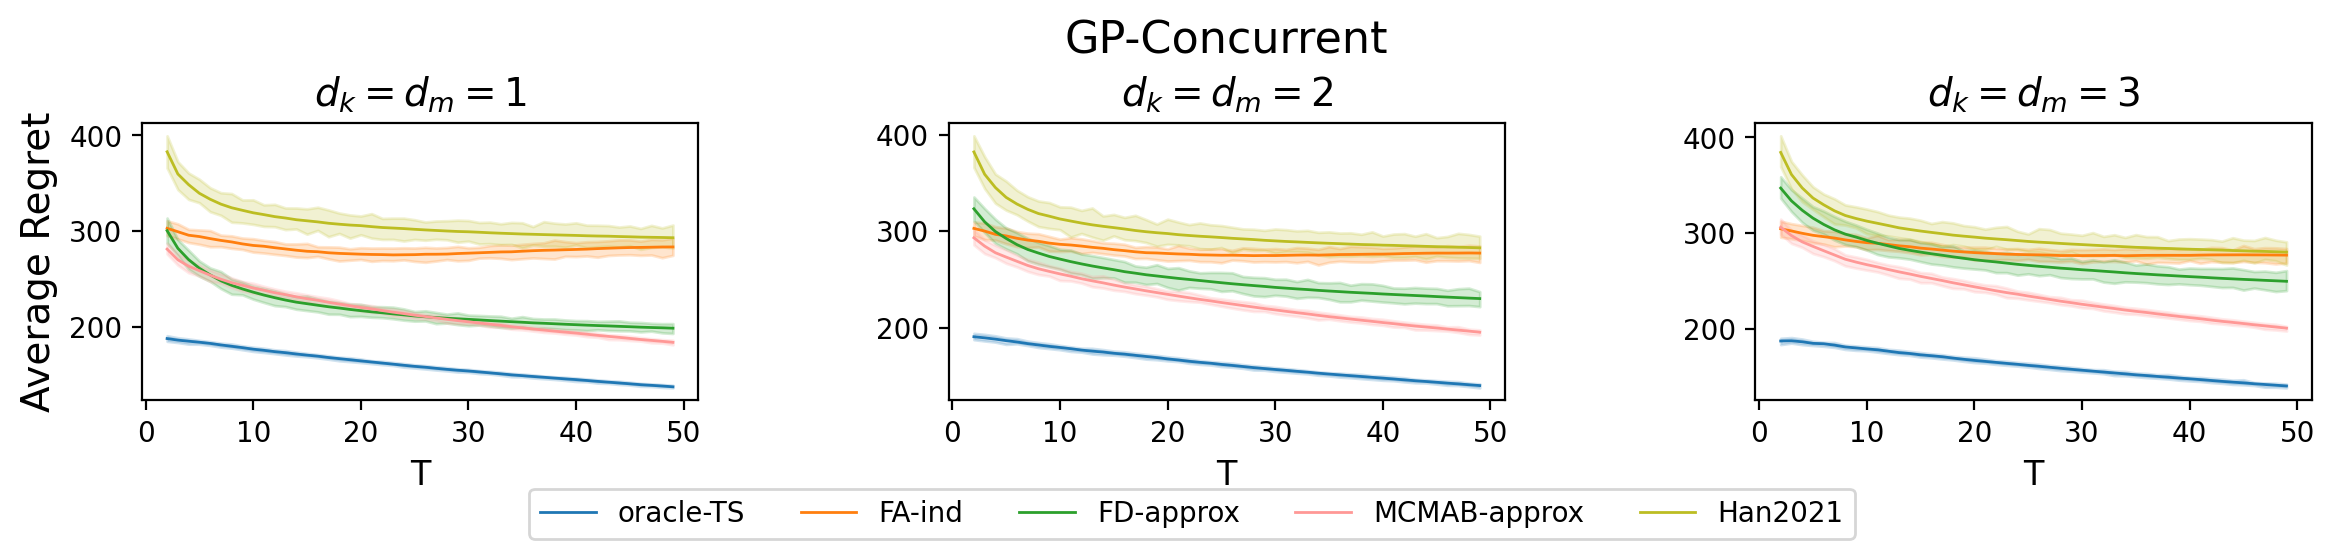}
    \caption{Simulation results for the concurrent nonlinear environment setting with different $d$ specifications, evaluating GP-based algorithms. Uninformative priors with zero mean and an RBF kernel are used. Shaded areas indicate the 95\% confidence interval.}
    \label{fig:GP_d}
\end{figure}

\begin{figure}[h]
    \centering
    \includegraphics[width = .75\linewidth]{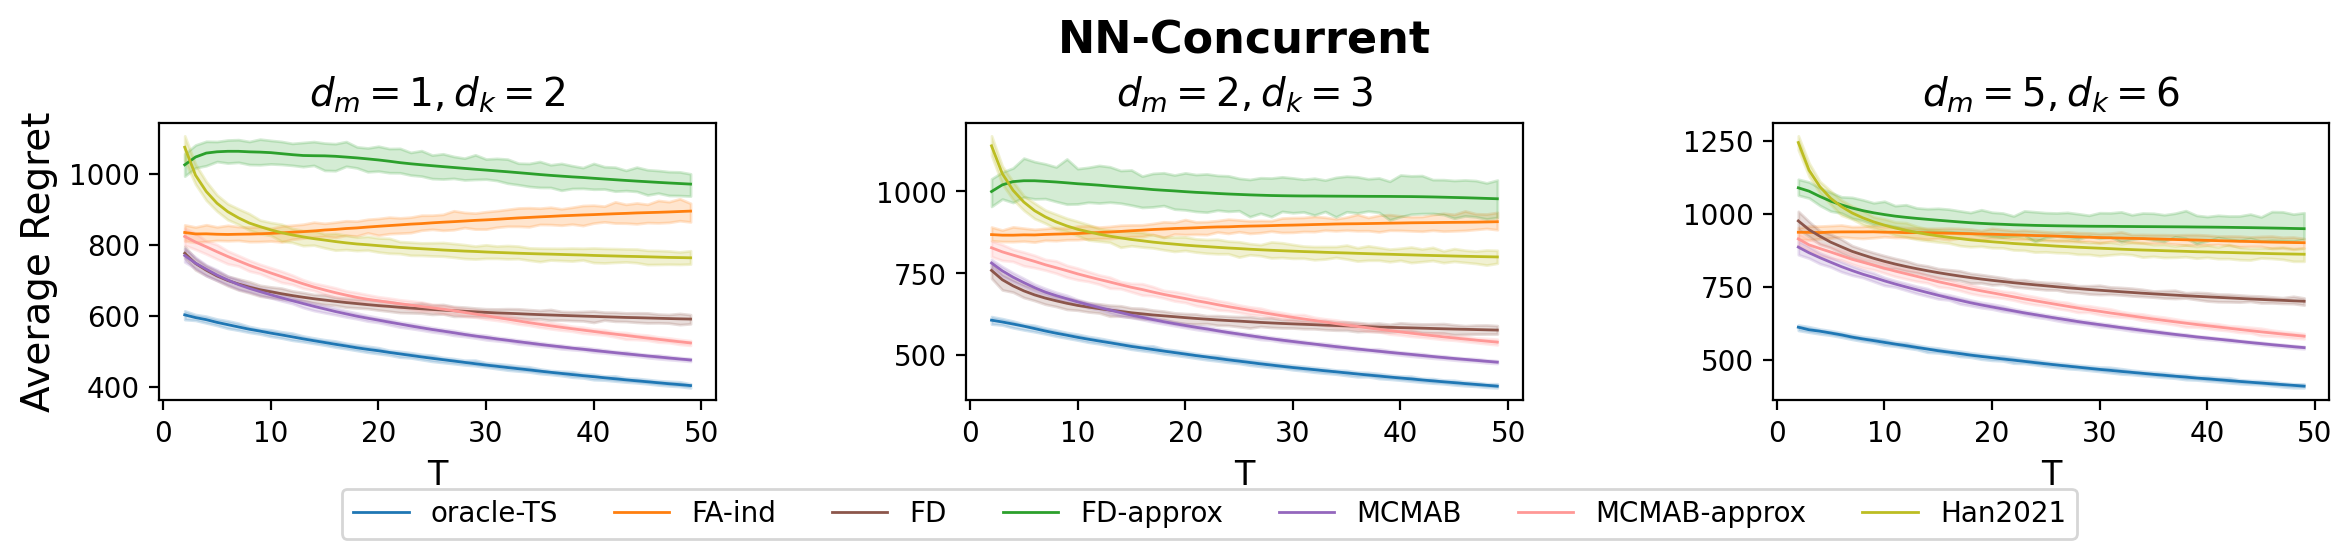}
    \caption{Simulation results for the concurrent nonlinear environment setting with different $d$ specifications, evaluating NN-based algorithms. We set a regularization parameter of 1, and a learning rate of.01 for all NN-based approaches.$(L=2, m=12)$ for NN-based algorithms in the setting with $(d_m =1,d_k=2)$,  $(L = 3, m=14)$ for NN-based algorithms in the setting with $(d_m = 2, d_k = 3)$, and $(L=3,m=20)$ for NN-based algorithms in the setting with $(d_m = 5, d_k = 6)$. Shaded areas indicate the 95\% confidence interval.}
    \label{fig:NN_d}
\end{figure}
