# Supplementary material for: Multi-Task Combinatorial Bandits for Budget Allocation
Source: arXiv:2409.00561 source file (2024-08-31)
Supplement: Supplementary file 3 [file 7.Appendix2.tex]

\section{Computational Efficient Variants} \label{efficient-variants}
In practice, for efficient deployment, it is not necessary to update $g$ at every decision time. Especially when observations are received in batches and decisions are made in batch mode, it is more appropriate to follow an offline training-online deployment framework. Specifically, at certain time points, we would update the posterior of the function $g$ based on all the information observed so far. Then, a function instance of $g$ is sampled and used as the prior for subsequent learning of $\vthe$ until the next time when $g$ is retrained and sampled. For example, Algorithm \ref{alg:TS-concurrent} outlines a computationally efficient variant of MCMAB tailored for concurrent scenarios. Here, $g$ is trained once daily before delivering recommendations. Algorithm \ref{alg:TS-sequential} describes an efficient variant for sequential settings, wherein $g$ is retrained only at the commencement of each new campaign.
\begin{algorithm}[!t]
\SetKwData{Left}{left}\SetKwData{This}{this}\SetKwData{Up}{up}
\SetKwFunction{Union}{Union}\SetKwFunction{FindCompress}{FindCompress}
\SetKwInOut{Input}{Input}\SetKwInOut{Output}{output}
\SetAlgoLined
\Input{Specification of $g$ and the corresponding prior; known parameters (i.e., $\sigma_\epsilon$, $\Cov$) of the hierarchical model
}
Set $\mH = \{\}$

\For{every decision point t}{ 
Update the posterior for $g$ as $\prob(g|\mH)$, according to the  hierarchical model \eqref{eqn:hierachical_model}\;

Sample a $\tilde{g} \sim \prob(g|\mH)$\;

\For{every campaign m}{
Given $\tilde{g}$, update the posterior for $\vthe_m$ as $\prob(\vthe_m|\tilde{g}, \mH)$\;

Sample an utility vector $\tilde{\vthe}_{m} \sim \prob(\vthe_m|\tilde{g}, \mH)$\; 

Take action $\boldsymbol{a}_{m,t} = argmax_{\boldsymbol{a}_{m,\cdot}\in\mathcal{S}_m} \sum_{k\in [K_m]}\tilde{\theta}_{m,k,a_{m,k,\cdot}}$\;

Receive reward $R_{m,t}$\;

Update the dataset as $\mH \leftarrow \mH \cup \{(m, \boldsymbol{a}_{m,t}, R_{m,t})\}$
}
}
\caption{Computational Efficient MCMAB-Concurrent}\label{alg:TS-concurrent}
\end{algorithm}

\begin{algorithm}[h]
\SetKwData{Left}{left}\SetKwData{This}{this}\SetKwData{Up}{up}
\SetKwFunction{Union}{Union}\SetKwFunction{FindCompress}{FindCompress}
\SetKwInOut{Input}{Input}\SetKwInOut{Output}{output}
\SetAlgoLined
\Input{Specification of $g$ and the corresponding prior; known parameters (i.e., $\sigma_\epsilon$, $\Cov$) of the hierarchical model
}
Set $\mH = \{\}$

\For{every campaign m}{ 
Update the posterior for $g$ as $\prob(g|\mH)$, according to the  hierarchical model \eqref{eqn:hierachical_model}\;

Sample a $\tilde{g} \sim \prob(g|\mH)$\;

\For{every decision time t}{

Given $\tilde{g}$, update the posterior for $\vthe_m$ as $\prob(\vthe_m|\tilde{g}, \mH)$\;

Sample an utility vector $\tilde{\vthe}_{m} \sim \prob(\vthe_m|\tilde{g}, \mH)$\; 

Take action $\boldsymbol{a}_{m,t} = argmax_{\boldsymbol{a}_{m,\cdot}\in\mathcal{S}_m} \sum_{k\in [K_m]}\tilde{\theta}_{m,k,a_{m,k,\cdot}}$\;

Receive reward $R_{m,t}$\;

Update the dataset as $\mH \leftarrow \mH \cup \{(m, \boldsymbol{a}_{m,t}, R_{m,t})\}$
}
}
\caption{Computational Efficient MCMAB-Sequential}\label{alg:TS-sequential}
\end{algorithm}
