# Supplementary material for: Multi-Task Combinatorial Bandits for Budget Allocation
Source: arXiv:2409.00561 source file (2024-08-31)
Supplement: Supplementary file 4 [file 9.Appendix4.tex]

\section{More Experimentation Details}

In the simulation study, we used uninformative priors for all GP- and NN-based approaches. Specifically, we assumed a Gaussian process prior with zero mean and an RBF kernel for all GP-based algorithms. For NN-based approaches, we rigorously follow the practice in \citet{zhang2020neural}, in which the initial weights for each layer except the output layer are sampled from $\mathcal{N}(0, 4/m)$, and the weights for the output layer are sampled from $\mathcal{N}(0,2/m)$. It is important to note that the performance of NN-based approaches is heavily dependent on their hyperparameters, which include the width $m$, depth $L$, regularization parameter, and learning rate. See \citet{yu2020hyper} for finetuning methods. For the experiments in Section \ref{synthetic}, we set $m = 12$, $L = 2$, a regularization parameter of 1, and a learning rate of.01 for all NN-based approaches.
